# Supplementary material for: SEA: Evaluating Sketch Abstraction Efficiency via Element-level Commonsense Visual Question Answering
Source: arXiv:2603.28363 source file (2026-03-30)
Supplement: Supplementary file 4 [file item.tex]

\begin{figure}[t]
\centering
% Row 1: Over-detail (g on/off)
\begin{subfigure}[t]{0.4\linewidth}
  \centering
  \includegraphics[width=\linewidth]{z_fig/reward_term/duck_67.png}
  \caption{Over-detail}
  \label{fig:overdetail}
\end{subfigure}
\hfill
% Row 1: Low-recog (g on/off)
\begin{subfigure}[t]{0.4\linewidth}
  \centering
  \includegraphics[width=\linewidth]{z_fig/reward_term/airplane_20.png}
  \caption{Low-recognizability}
  \label{fig:lowrecog}
\end{subfigure}

% Row 2: Table (inside figure)
\begin{subfigure}[t]{0.98\linewidth}
\centering
\scriptsize
\setlength{\tabcolsep}{3pt}

\begin{tabular}{lcccc}
\toprule
 & $v{=}V/E$ & $P$ & SEA (w/ $g$) & SEA (w/o $g$) \\
\midrule
Over-detail & 0.692 & 0.631 & -0.428 & +0.168 \\
Low-recog.  & 0.600 & 0.178 & -0.925 & +0.027 \\
\bottomrule
\end{tabular}
\caption{Numerical summary of the two examples.}
\label{fig:example_table}
\end{subfigure}
\vspace{-3pt}
\caption{Qualitative examples illustrating the role of the centered gate $g(\cdot)$. 
When $v>P$, $g(\cdot)<0$ suppresses SEA; removing $g(\cdot)$ yields misleadingly higher scores.}
\label{fig:gate_examples}
\end{figure}
